# Supplementary material for: A new measurement of the permanent electric dipole moment of $^{129}$Xe using $^{3}$He comagnetometry and SQUID detection
Source: arXiv:1902.02864 ancillary file (2019-02-07)
Supplement: Supplementary file 1 [file HeXe2017Supplement.pdf]

# Supplemental material for: A new measurement of the permanent electric dipole moment of $^{129}$Xe using $^{3}$He comagnetometry and SQUID detection

N. Sachdeva,[1] I. Fan,[2] E. Babcock,[3] M. Burghoff,[2] T. E. Chupp,[1] S. Degenkolb,[1,4] P. Fierlinger,[5] E. Kraegeloh,[5,1] W. Kilian,[2] S. Knappe-Grüneberg,[2] F. Kuchler,[5,6] T. Liu,[2] M. Marino,[5] J. Meinel,[5] Z. Salhi,[3] A. Schnabel,[2] J. T. Singh,[7] S. Stuiber,[5] W. A. Terrano,[5] L. Trahms,[2] and J. Voigt[2]

[1]*Department of Physics, University of Michigan, Ann Arbor, Michigan 48109, USA*
[2]*Physikalisch-Technische Bundesanstalt (PTB) Berlin, 10587 Berlin, Germany*
[3]*Jülich Center for Neutron Science, 85748 Garching, Germany*
[4]*Institut Laue-Langevin, 38042 Grenoble, France*
[5]*Excellence Cluster Universe and Technische Universität München, 85748 Garching, Germany*
[6]*TRIUMF, Vancouver, British Columbia V6T 2A3, Canada*
[7]*National Superconducting Cyclotron Laboratory and Department of Physics & Astronomy, Michigan State University, East Lansing, Michigan 48824, USA*

(Dated: February 7, 2019)

## COMAGNETOMETER SENSITIVITY TO MAGNETIC FIELD PERTURBATIONS

Ideally, a comagnetometer EDM measurement uses two species with identical responses to magnetic perturbations and very different sensitivities to CPV effects. We have chosen $^{129}$Xe and $^{3}$He, two $F = 1/2$ atoms. Note that both $^{129}$Xe and $^{3}$He have negative magnetic moments, *i.e.* the magnetic moment is opposite the total angular momentum $\vec{F}$; therefore, for positive $\vec{d}$ (parallel to $\vec{F}$), the precession frequency will decrease when $\vec{E}$ is parallel to $\hat{B}$ ($\vec{E}\cdot\hat{B} > 0$). Thus, an EDM contributes a frequency shift to each species given by

$$\omega_{d_{\rm Xe}} = -\frac{2d_A(^{129}{\rm Xe})}{\hbar}\vec{E}\cdot\hat{B} \qquad \omega_{d_{\rm He}} = -\frac{2d_A(^{3}{\rm He})}{\hbar}\vec{E}\cdot\hat{B}, \tag{1}$$

where the $^{3}$He EDM is strongly suppressed because diamagnetic atoms' sensitivity to CPV is approximately proportional to $Z^2$ [1].

Potential systematic effects, *i.e.* false-EDM signals, arise because the two species have different responses to the magnetic field environment due to chemical shifts, diffusion in magnetic field gradients, and species-dependent self and cross-species interactions. Additionally, the apparatus that measures the spin precession rotates with the Earth, adding an offset to the precession frequencies. Taking these into account, the two species' precession frequencies can be summarized as

$$\omega_{\rm Xe} = \omega_{d_{\rm Xe}} + \gamma'_{\rm Xe}(1-\delta_{\rm Xe})\langle B\rangle_{\rm Xe} + \omega^{sd}_{\rm Xe} + \vec{\Omega}\cdot\hat{B} \tag{2}$$

$$\omega_{\rm He} = \omega_{d_{\rm He}} + \gamma'_{\rm He}(1-\delta_{\rm He})\langle B\rangle_{\rm He} + \omega^{sd}_{\rm He} + \vec{\Omega}\cdot\hat{B}, \tag{3}$$

where
$\gamma'_{\rm Xe/He} = \frac{2\mu_{\rm Xe/He}}{\hbar}\sigma_{\rm Xe/He}$ are the shielded gyromagnetic ratios of the atoms;
$\mu_{\rm Xe/He}$ are nuclear magnetic moments;
$\sigma_{\rm Xe/He}$ are the atomic diamagnetic shielding factors;
$\delta_{\rm Xe/He}$ are species-dependent chemical shifts which depend on pressure, temperature, surrounding materials, etc.;
$\langle B\rangle_{\rm Xe/He}$ is the magnetic field averaged over space and time in the presence of second- and higher-order gradients, which are not identically averaged by the two species due to different diffusion constants;
$\omega^{sd}_{\rm Xe/He}$ is the species dependent shift;
$\vec{\Omega}$ is the Earth's angular velocity, and $\vec{\Omega}\cdot\hat{B}$ is its projection onto $\vec{B}$.
The comagnetometer frequency is defined as the combination

$$\omega_{\rm co} \equiv \omega_{\rm Xe} - R\omega_{\rm He}, \tag{4}$$

where $R = 1/2.7540816$ is the nominal ratio of shielded gyromagnetic ratios. Using Eqs. 2 and 3, with $\omega_d \equiv \omega_{d_{\rm Xe}} - R\omega_{d_{\rm He}}$, the comagnetometer frequency is

$$\omega_{\rm co} = \omega_d + \left[\gamma'_{\rm Xe}(1-\delta_{\rm Xe})\langle B\rangle_{\rm Xe} - R\gamma'_{\rm He}(1-\delta_{\rm He})\langle B\rangle_{\rm He}\right] + (\omega^{sd}_{\rm Xe} - R\omega^{sd}_{\rm He}) + (1-R)\vec{\Omega}\cdot\hat{B}. \tag{5}$$

Further insight is gained by considering the lowest-order response to changes of $\langle B\rangle_{\mathrm{Xe/He}}$ and $\delta_{\mathrm{Xe/He}}$:

$$\langle B\rangle_{\mathrm{Xe/He}} = B + \Delta B^{\mathrm{dif}}_{\mathrm{Xe/He}},$$

where $B$ is the magnetic field spatially averaged over the cell and $\Delta B^{\mathrm{dif}}_{\mathrm{Xe/He}}$ is the difference of the field actually averaged by the two species.

$$R\ = R^0 + \Delta R = \frac{\gamma'_{\mathrm{Xe}}(1-\delta_{\mathrm{Xe}})}{\gamma'_{\mathrm{He}}(1-\delta_{\mathrm{He}})},$$

where

$$R^0 = \frac{\gamma'_{\mathrm{Xe}}}{\gamma'_{\mathrm{He}}}; \qquad \Delta R \approx R^0\left(\delta_{\mathrm{He}} - \delta_{\mathrm{Xe}}\right). \tag{6}$$

Therefore, Eq. 5 reduces to

$$\begin{aligned}\omega_{\mathrm{co}} \approx\ & \omega_d \\ & + (1-R)\,\vec{\Omega}\cdot\hat{B} \\ & - \gamma'_{\mathrm{He}}\Delta R B \\ & + \gamma'_{\mathrm{Xe}}\left(\Delta B^{\mathrm{dif}}_{\mathrm{Xe}} - \Delta B^{\mathrm{dif}}_{\mathrm{He}}\right) \\ & + \left(\omega^{sd}_{\mathrm{Xe}} - R\omega^{sd}_{\mathrm{He}}\right).\end{aligned} \tag{7}$$

The $2^{\mathrm{nd}}$ through $4^{\mathrm{th}}$ terms in Eq. 7 indicate the sensitivity of $\omega_{\mathrm{co}}$ to the magnitude, direction, and gradients of the magnetic field. Any correlation of these with the HV may cause a false-EDM signal. Such correlations are expected from possible leakage currents that flow across the cell, magnetization induced by charging currents that flow when the HV is changed, and motion of the measurement cell due to electrostatic forces that change with the HV. Our approach to estimating false-EDM signals is based on auxiliary measurements that measure the comagnetometer frequency response to amplified leakage and charging currents, gradients, and cell motion, which are scaled to the observed maximum of these parameters monitored during the experiment.

In Table I, we show how the systematic error from false-EDM effects were determined from auxiliary measurements. The comagnetometer drift is not a direct coupling to the magnetic field and is addressed in the next section.

| | Leakage current | Charging current | Cell translation | Cell rotation | External dipole (loop test) |
|---|---|---|---|---|---|
| Auxiliary measurement | Single turn $\pm 0.1$–$1\ \mu$A | $\pm 10$–$20\ \mu$A | N/A | $\pm 5^\circ$ | Loop attached to electrode 0–100 $\mu$A |
| Measured linear dependence | $\frac{1}{2\pi}\frac{\partial\omega_{\mathrm{co}}}{\partial I} = (1.32\pm0.93)$ Hz/A | $\frac{1}{2\pi}\frac{\partial\omega_{\mathrm{co}}}{\partial I} = (-0.3\pm1.2)$ mHz/A | $\frac{1}{2\pi}\frac{\partial\omega_{\mathrm{co}}}{\partial z}$ $\leq 90$ nHz/m | $\frac{1}{2\pi}\frac{\partial\omega_{\mathrm{co}}}{\partial\theta}$ $\leq 1.6$ $\mu$Hz/rad | $\frac{1}{2\pi}\frac{\partial\omega_{\mathrm{co}}}{\partial\omega_{\mathrm{He}}} = (-1.55\pm0.28)\times10^{-3}$ |
| Observed HV-correlated maximum | $I_{\mathrm{leak}} = 97$ pA | $I_{\mathrm{charge}} = 19$ nA | $\delta z \leq 30\ \mu$m | $\delta\theta \leq 33\ \mu$rad | $\delta\omega^{HV}_{\mathrm{He}} = (-181.4\pm124.4)$ nHz |
| False EDM ($e$cm) | $1.2\times10^{-28}$ | $1.7\times10^{-29}$ | $1.9\times10^{-30}$ | $4.2\times10^{-29}$ | $2.6\times10^{-28}$ |

TABLE I. Systematic effects arising from HV-correlated magnetic field perturbations that lead to false-EDM signals. Each column corresponds to an HV-correlated effect. The HV-correlated frequency shift is found from the linear dependence multiplied by the maximum observed change during the EDM measurements. The false EDM is the 68% c.l. upper limit of frequency shift multiplied by the conversion factor $7\times10^{-28}$ $e$cm/nHz. The loop test measured $\frac{\partial\omega_{\mathrm{co}}}{\partial\omega_{\mathrm{He}}}$ and is most sensitive to the higher-order gradient contribution $\gamma'_{\mathrm{Xe}}\left(\Delta B^{\mathrm{dif}}_{\mathrm{Xe}} - \Delta B^{\mathrm{dif}}_{\mathrm{He}}\right)$. In lieu of a direct auxiliary measurement of cell translation, this was used to set an upper limit on the false EDM due to cell translation with respect to a gradient source external to the cell, and the total cell translation false EDM added this to the limit on translation coupled to the $B$ dependence.

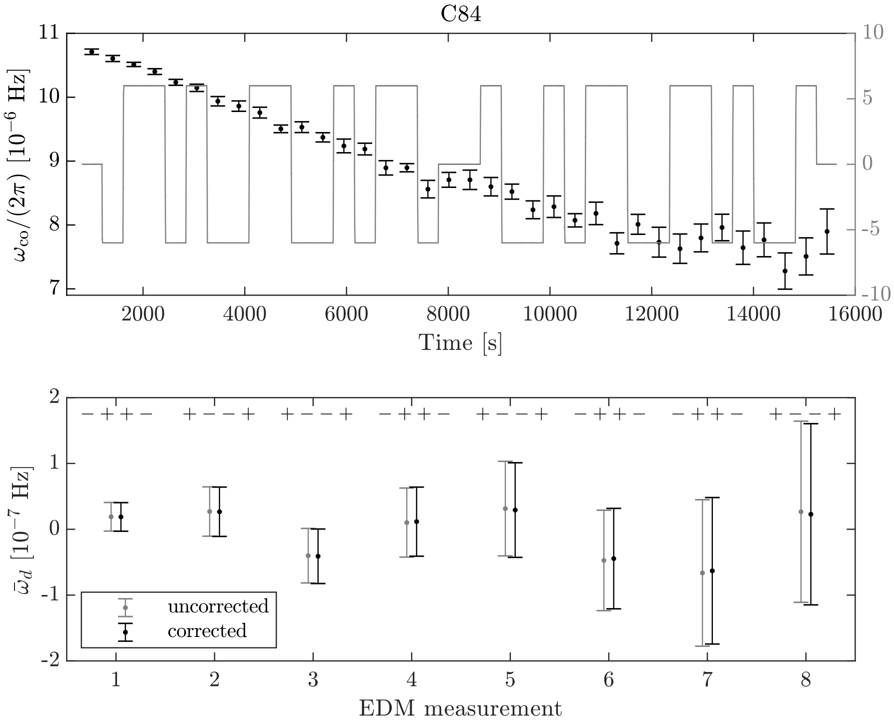


FIG. 1. Top: Segment frequencies $\omega_{co}$ (left axis) and the HV pattern (right axis) for a single cell-filling run. The offset of the comagnetometer frequency is due largely to the combination of the chemical shift and Earth's rotation, which are compensated by combining segment frequencies in combinations of two or more segments with opposite HV. See Eq. 7 and the following discussion. Bottom: Four-segment EDMs, which compensate linear drifts; (left/gray) uncorrected and (right/black) corrected for higher order drifts. As shown in Table II, the drift correction reverses with the polarity of the first HV segment in the sequence of four and increases in magnitude later in the run.

## COMAGNETOMETER DRIFT CORRECTION

Uncompensated drift of $\omega_{co}$ would appear as a false EDM due to the frequency shift between segments with opposite $\vec{E}\cdot\hat{B}$. Fig. 1 shows the segment frequencies $\omega_{co}$ as a function of time for a single run, illustrating the typical comagnetometer drift of a few $\mu$Hz over the course of the run. Segment-to-segment drift was, by experiment design, comparable to or less than the statistical error of $\omega_{co}$ for a segment. These drifts are predominantly due to effects of residual longitudinal magnetization, and recent studies have shown that these drifts are dominated by the combination of two effects: a phase shift induced by the cell-shape dependent torque on the longitudinal magnetization of one species due to the precessing magnetization of the same species [2] and the additional effective static magnetic field exerted on one species due to contact interactions during collisions with the other [2, 3]. The drifts are expected to be a combination of exponential decays due to the $T_1$ decay of longitudinal magnetization of the two species, assumed to be 5,000–10,000 seconds.

The drifts for all runs were monotonic and accurately parametrized by polynomials of up to $4^{\text{th}}$ order. The HV reversal pattern shown in Table II was designed to cancel drifts characterized by polynomials of order $n$ for sequences of $N = 2^{n+1}$ segments. For example, a sequence of time-dependent frequencies plus $\omega_d$ can be described by

$$\omega_{co}(t_i) = \omega_d + k_0 + k_1 t_i + k_2 t_i^2 + k_3 t_i^3 + \dots, \tag{8}$$

where $t_i = i\Delta t$. The average of $N \geq 1$ consecutive frequencies starting at segment $i_0$, with $i_0 = 1, 1+N, 1+2N, \dots$, is

$$\bar{\omega}_d = \frac{1}{N}\sum_{i=i_0}^{i_0+N} S_i^{EB}\omega_{co} = -\frac{2d|E|}{\hbar} + c_1 k_1 \Delta t + c_2 k_2 \Delta t^2 + \dots + c_n k_n \Delta t^n, \tag{9}$$

where $S_i^{EB} = \mathrm{sgn}(\hat{E}\cdot\hat{B})$ and

$$c_1 = \frac{1}{N}\sum_{i=i_0}^{i_0+N} S_i^{EB} i = \frac{1}{N}\left[i_0 - (i_0+1) - (i_0-2) + (i_0+3) + \ldots\right],$$
$$c_2 = \frac{1}{N}\sum_{i=i_0}^{i_0+N} S_i^{EB} i^2, \qquad \text{etc.} \tag{10}$$

For $N = 4$, $c_1 = 0$, for $N = 8$, $c_2 = c_1 = 0$, *etc.*. The values of $c_{2-4}$ for the four-segment sequence ($N = 4$) are given in Table II. Because the signals decay, the frequency uncertainty per segment increases over time. Since the combination of $N$ segments for an EDM measurement is an unweighted average, using larger $N$ sequences result in larger statistical error in the final weighted average of EDM measurements. Because the observed drifts were mostly linear, a $N = 4$ sequence was used in the analysis and the correction for higher-order drifts was small compared to the statistical error.

| Segment | $S^{EB}$ | $c_2$ | $c_3$ | $c_4$ | Segment | $S^{EB}$ | $c_2$ | $c_3$ | $c_4$ |
|---|---|---|---|---|---|---|---|---|---|
| 0 | 0 | | | | 18 | 0 | | | |
| 1 | + | 1 | 7.5 | 40 | 19 | − | −1 | −61.5 | −2524 |
| 2 | − | | | | 20 | + | | | |
| 3 | − | | | | 21 | + | | | |
| 4 | + | | | | 22 | − | | | |
| 5 | − | −1 | −19.5 | −256 | 23 | + | 1 | 73.5 | 3604 |
| 6 | + | | | | 24 | − | | | |
| 7 | + | | | | 25 | − | | | |
| 8 | − | | | | 26 | + | | | |
| 9 | − | −1 | −31.5 | −664 | 27 | + | 1 | 85.5 | 4876 |
| 10 | + | | | | 28 | − | | | |
| 11 | + | | | | 29 | − | | | |
| 12 | − | | | | 30 | + | | | |
| 13 | + | 1 | 43.5 | 1264 | 31 | − | −1 | −97.5 | −6340 |
| 14 | − | | | | 32 | + | | | |
| 15 | − | | | | 33 | + | | | |
| 16 | + | | | | 34 | − | | | |
| 17 | 0 | | | | 35 | 0 | | | |

TABLE II. HV pattern and weights $c_i$ for polynomial fit coefficients $k_i$ used in higher-order drift corrections for 18 and 36 segments of a run starting with +HV. For runs starting with −HV, the patterns and coefficients are reversed (multiply by −1).

For each run, the comagnetometer frequencies were fit to $2^{\text{nd}}$, $3^{\text{rd}}$ and $4^{\text{th}}$ order polynomials, and the $F$-test statistic was calculated for each increasing polynomial order. Table III shows the integrated probability $\int_{F_{\min}}^{\infty} P(F)dF$ for adding a quadratic, cubic, and quartic term for all runs. For each run, a correction was applied to $\bar{\omega}_d$ for each polynomial order if the integrated probability exceeded a specific threshold. The threshold of 0.6 was chosen by using blinded frequencies based on the range over which the uncertainty of the correction was relatively constant. Since the frequencies were blinded, the EDM was offset by different amounts for the two cells and the final correction was therefore determined from the difference of corrected and uncorrected unblinded EDMs, which are shown as a function of threshold in Table IV . The bottom panel of Fig. 1 shows $\bar{\omega}_d$ for a single run along with the corrections for higher order drift. The corrections alternate with the HV polarity at the start of the four-segment sequence, but do not fully cancel for a run. For a threshold of 0.6, the correction was $(-0.08 \pm 0.66) \times 10^{-27}\, e\,\text{cm}$, where the uncertainty is a statistical error based on the polynomial fits to the segment frequencies for each run.

| Run | Cell | Quadratic | Cubic | Quartic |
|---|---|---|---|---|
| C82 | PP2 | 1.00 | 0.86 | 0.82 |
| C83 | PP2 | 0.98 | 0.85 | 0.08 |
| C84 | PP2 | 1.00 | 0.98 | 0.45 |
| C85 | PP2 | 0.90 | 0.48 | 0.14 |
| C86 | PP1 | 0.98 | 0.89 | 0.86 |
| C89 | PP1 | 0.14 | 0.57 | 0.47 |
| C91 | PP1 | 1.00 | 0.34 | 0.65 |
| C92 | PP1 | 1.00 | 0.73 | 0.70 |
| C93 | PP2 | 1.00 | 0.64 | 0.07 |
| C02 | PP2 | 1.00 | 0.04 | 0.94 |
| C08 | PP2 | 0.99 | 1.00 | 0.01 |
| C10 | PP1 | 1.00 | 0.89 | 0.86 |
| C12 | PP2 | 0.99 | 0.37 | 0.08 |
| C13 | PP2 | 0.25 | 1.00 | 0.40 |
| C14 | PP2 | 1.00 | 0.72 | 0.52 |
| C15 | PP1 | 0.99 | 0.85 | 0.78 |

TABLE III. $\int_{F_{\rm min}}^{\infty} P(F)dF$ by run for quadratic, cubic, and quartic terms in the polynomial fit. For C13, quadratic and cubic terms were included for the drift correction.

| $P_{\rm thres.}$ | $d_{\rm cor}$ ($10^{-27}$ $e$ cm) | $\sigma_{d_{\rm cor}}$ ($10^{-27}$ $e$ cm) | correction ($10^{-27}$ $e$ cm) | $\sigma_{\rm cor}$ ($10^{-27}$ $e$ cm) |
|---|---|---|---|---|
| 0 | −0.42 | 2.59 | −0.76 | 1.13 |
| 0.2 | −0.29 | 2.55 | −0.63 | 1.04 |
| 0.4 | 0.20 | 2.43 | −0.14 | 0.69 |
| 0.5 | 0.21 | 2.43 | −0.13 | 0.69 |
| 0.6 | 0.26 | 2.42 | −0.08 | 0.66 |
| 0.8 | 0.24 | 2.36 | −0.10 | 0.36 |
| no correction | 0.34 | 2.33 | N/A | N/A |

TABLE IV. Results for the corrected EDM as a function of the threshold for $\int_{F_{\rm min}}^{\infty} P(F)dF > P_{\rm thres.}$. The correction is the difference between the corrected EDM $d_{\rm cor}$ and the uncorrected EDM $d_{\rm uncor}$, and the uncertainty of the correction $\sigma_{\rm cor}$ is estimated such that $\sigma_{d_{\rm cor}} = \sqrt{\sigma^2_{d_{\rm uncor}} + \sigma^2_{\rm cor}}$.

[1] V. V. Flambaum and J. S. M. Ginges, Phys. Rev. A **65**, 032113 (2002).
[2] W. A. Terrano, J. Meinel, N. Sachdeva, T. Chupp, S. Degenkolb, P. Fierlinger, F. Kuchler, and J. T. Singh, (2018), arXiv:1807.11119 [physics.atom-ph].
[3] M. E. Limes, N. Dural, M. V. Romalis, E. L. Foley, T. W. Kornack, A. Nelson, and L. R. Grisham, (2018), arXiv:1805.11578.
